# Supplementary material for: Dynamic melting and condensation of topological dislocation modes
Source: arXiv:2210.15661 ancillary file (2023-11-02)
Supplement: Supplementary file 1 [file suppl.pdf]

# Supplemental Material: Dynamic melting and condensation of topological dislocation modes

Sanjib Kumar Das[1] and Bitan Roy[1]
[1]*Department of Physics, Lehigh University, Bethlehem, Pennsylvania, 18015, USA*
(Dated: September 23, 2023)

In this Supplemental Material, (a) we present additional numerical results [Sec. S1, and Figs. S1 and S2], (b) comparison of the survival probability of a single dislocation mode across a sudden quench with $P(t)$ for the pure state with large ramp speed $\alpha$ [Sec. S2 and Fig. S3], and (c) analyze the probability of finding the dislocation modes in a mixed state (denoted by HF$'$) initially prepared in the M phase [Sec. S3].

## S1. ADDITIONAL NUMERICAL RESULTS

In the main manuscript we made the following claims regarding the phase diagram of the model static Hamiltonian $H$ [Eq. (2)]. It supports (a) a topological insulator (TI) with the band inversion at the $\Gamma$ point of the Brillouin zone (BZ) for $0 < m_0/t_0 < 2$, (b) a TI with the band inversion at the M point of the BZ for $-2 < m_0/t_0 < 0$, and (c) trivial or normal insulators for $m_0/t_0 > 2$ and $m_0/t_0 < 2$. Here we justify these claims from the band structure of $H$, where besides showing the energy eigenvalues along various high symmetry lines in the BZ, we also display the orbital polarization (in red and blue) of the corresponding wavefunctions for the valence and conduction bands along those high symmetry lines. The results are displayed in Fig. S1. Throughout we set $t = t_0 = 1$.

Notice that in the normal or trivial insulating phases, the orbital polarization of the valence and conduction bands remains unchanged in the entire BZ. By contrast, the orbital polarization changes along the $\Gamma - \mathrm{X}$ and $\mathrm{M} - \Gamma$ lines for $m_0 = 0.1$, confirming that the band inversion takes place near the $\Gamma$ point. For $m_0 = -1.0$ the orbital polarization changes along the $\mathrm{X}-\mathrm{M}$ and $\mathrm{M}-\Gamma$ lines, confirming that the band inversion takes place around the M point of the BZ.

In the main manuscript, we also claimed that in a half-filled system the average electronic density on any site $\langle N_i \rangle = 1$, irrespective of whether the system supports any dislocation mode or not, where $i$ is the site index. Moreover, under real time ramp $\langle N_i(t) \rangle = 1$ at any instant of time $(t)$ for arbitrary values of $\alpha$, $m_i$ and $m_f$. This

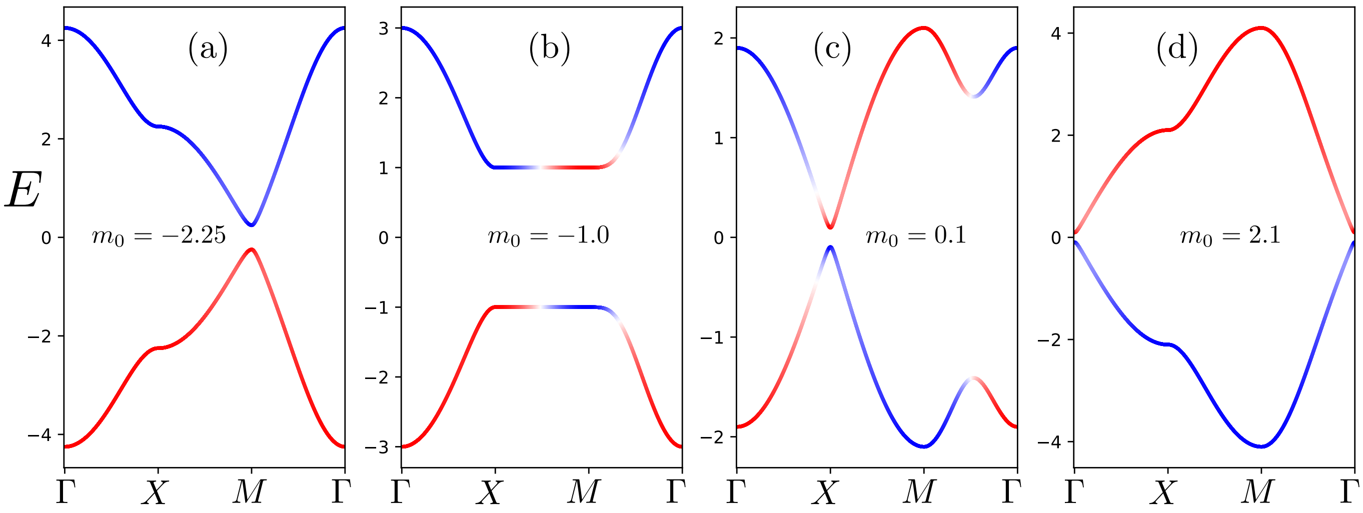


Figure S1. Band structure of the model Hamiltonian (see Eq. (2) of main manuscript) is shown along the high symmetry path in the BZ for various values of $m_0$. Here we take the path $\Gamma \to \mathrm{X} \to \mathrm{M} \to \Gamma$ in the BZ, where $\Gamma = (0, 0)$, $X = (\pi, 0)/a$ and $\mathrm{M} = (\pi, \pi)/a$, and $a$ is the lattice spacing. The orbital polarization of the wavefunctions for the valence and conduction bands are shown in red and blue. For (a) $m_0 = -2.25$ and (d) $m_0 = 2.1$ system describes normal insulators with no band inversion, but with band minima near the M and $\Gamma$ points respectively. For (b) $m_0 = -1.0$ and (c) $m_0 = 0.1$, the system describes topological insulators with the band inversion near the M and $\Gamma$ points, respectively. For details see Sec. S1. Here $E$ is energy, and throughout we set $t = t_0 = 1$.

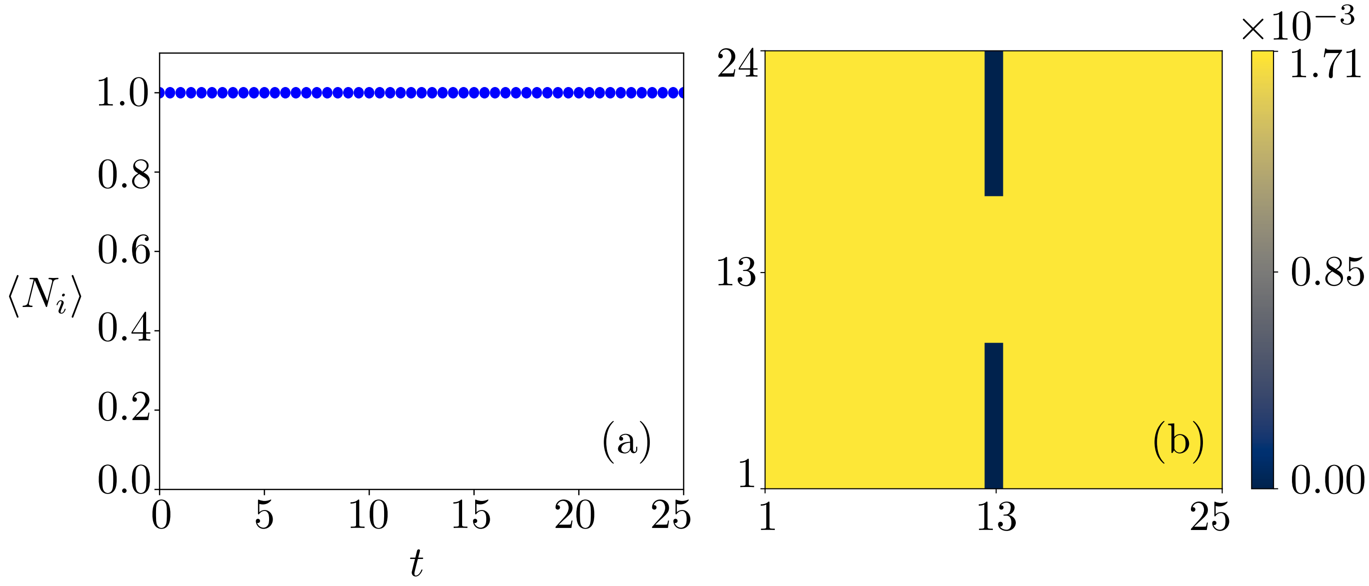


Figure S2. (a) Time dependence of the average electronic density $\langle N_i(t)\rangle$ in a half-filled system for any value of $i$ (site index) for any values of $\alpha$, $m_i$ and $m_f$. (b) Correspondingly, the site resolved LDOS $D_i(t)$ shows constant value for all the sites in the entire system (independent of $\alpha$, $m_i$ and $m_f$ and $t$). Both $D_i(t)$ and $\langle N_i\rangle = ND_i(t)$ are computed from the density matrix $\rho(t)$. Here $N$ is the number of sites in the system.

outcome is further strengthened by the site resolved LDOS, $D_i(t)$, computed from Eq. (5) of the main manuscript. The average electronic density at each site is given by $\langle N_i(t)\rangle = ND_i(t)$, where $N$ is the total number of lattice sites in the system. The results are shown in Fig. S2.

## S2. SURVIVAL PROBABILITY OF A DISLOCATION MODE ACROSS A SUDDEN QUENCH

The survival probability of a single dislocation mode after a sudden quench from the translationally active M phase to any one of the translationally inert insulating phases is given by [1, 2]

$$S_p(t) = \Big| \sum_{n=1}^{2N} |\langle \Psi_{\rm dis}^{\rm initial} | \Phi_n^{\rm final}\rangle|^2 e^{-iE_n t} \Big|^2, \tag{S1}$$

where $|\Psi_{\rm dis}^{\rm initial}\rangle$ is one of the initial (set by $m_0 = m_i$) dislocation modes, realized in the M phase of $H$ [Eq. (2) of the main manuscript], and $|\Phi_n^{\rm final}\rangle$ is the wavefunction of the postquench Hamiltonian (characterized by $m_0 = m_f$), with eigenenergy $E_n$. Here $N$ is the total number of sites in the system, accommodating total $2N$ number of states. The time evolutions of $S_p(t)$ for various choices of $m_f$ are shown in Fig. S3.

We find that for a fixed $m_i$ (ensuring that the system is initially in the translationally active M phase that supports dislocation modes) and for any $m_f$, the time evolution of the survival probability $S_p(t)$ of a single dislocation mode across a sudden quench matches *exactly* with the probability $P(t)$ [see Eq. (4) of the main manuscript] of finding the dislocation mode at any time $t > 0$ in the pure state initially prepared for a single dislocation mode when the ramp speed, characterized by $\alpha$ [see Eq. (3) of the main manuscript], is sufficiently large (large $\alpha$). Notice that a large $\alpha$ closely mimics a sudden quench.

## S3. PROBABILITY OF DISLOCATION MODES IN A MIXED STATE DURING DYNAMIC MELTING

The initial density matrix in the HF′ state, containing $N+1$ number of fermions, where $N$ is the number of lattice sites in the system capable of accommodating total $2N$ number of fermions, in the presence of a pair of

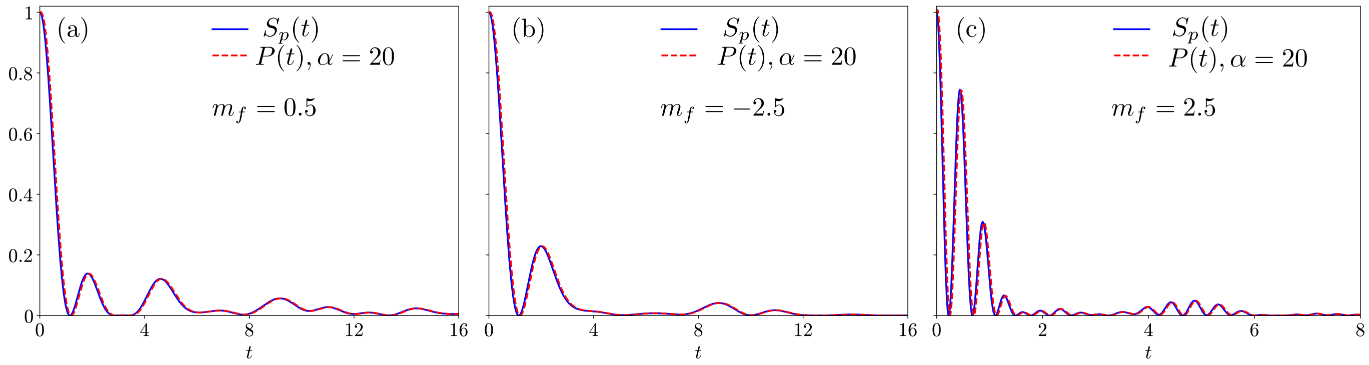


Figure S3. Comparison between the survival probability $S_p(t)$ and the time evolution of probability $P(t)$ of finding a single dislocation mode in a pure state of a single dislocation mode, for a fixed $m_i = -1$ (yielding the M phase) and various choices of $m_f$ (quoted in each subfigure), yielding different candidates for translationally inert insulators [see Fig. 1(c) showing the phase diagram of the Hamiltonian $H$ from Eq. (2) of the main manuscript]. Clearly, for $\alpha = 20$ (a large ramp speed, closely mimicking a sudden quench), $P(t)$ almost coincides with the $S_p(t)$. See also Sec. S2.

dislocation-antidislocation, constructed from the eigenstates $|\Psi_i\rangle$ of the initial Hamiltonian with energy $E_i$ is

$$\rho(0) = \frac{1}{N+1} \sum_{i=1}^{N+1} |\Psi_i\rangle \langle\Psi_i| \,. \tag{S2}$$

Among $N+1$ states, there are two near zero energy dislocation modes, denoted by $\left|\Psi_i^{\rm dis}\right\rangle$ with $i = 1, 2$. The probability of finding any occupied state $|\Psi_j\rangle$ (including the dislocation modes) is (see also Eq. (6) of the main manuscript)

$$P(0) = \langle\Psi_j| \rho |\Psi_j\rangle = \frac{1}{N+1} \sum_{i=1}^{N+1} \langle\Psi_j|\Psi_i\rangle \langle\Psi_i|\Psi_j\rangle = \frac{1}{N+1} \sum_i \delta_{ji}\delta_{ij} = \frac{1}{N+1}. \tag{S3}$$

Probability of finding the combined wavefunction of the dislocation modes, defined as $\left|\Psi^{\rm dis}\right\rangle = (\left|\Psi_1^{\rm dis}\right\rangle + \left|\Psi_2^{\rm dis}\right\rangle)/\sqrt{2}$, is also equal to $(N+1)^{-1}$. This is the maximal probability of finding the dislocation modes in the HF$'$ state when the real time ramp causes dynamic melting of these modes. See Fig. 2(bottom) of the main manuscript.

In our formalism, the density matrix $\rho(t)$ is a $2N \times 2N$ Hermitian operator with $2N$ number of real positive semi-definite eigenvalues $\rho_i(t)$, such that $\sum_{i=1}^{2N} \rho_i(t) = 1$ at any time. Therefore, the set of eigenvectors of $\rho(t)$, namely $\{\phi_i(t)\}$ form a complete orthonormal set of basis vectors at any time $t$. Therefore, $|\Psi\rangle$ can be expressed as the linear combination of the basis vectors $\{\phi_i(t)\}$ according to $|\Psi\rangle = \sum_{i=1}^{2N} C_i(t) |\phi_i(t)\rangle$, where $\sum_{i=1}^{2N} |C_i(t)|^2 = 1$.

The probability of finding the dislocation mode at any time $t$ can then be written as

$$P(t) = \langle\Psi| \rho(t) |\Psi\rangle = \sum_{i,j=1}^{2N} C_i(t)^* C_j(t) \langle\phi_i(t)| \rho(t) |\phi_j(t)\rangle = \sum_{i,j=1}^{2N} C_i^*(t) C_j(t) \rho_j(t) \langle\phi_i(t)|\phi_j(t)\rangle = \sum_{i=1}^{2N} |C_i(t)|^2 \rho_i(t). \tag{S4}$$

The minimum value of $P(t)$ can be obtained for $C_i(t) = 1/\sqrt{2N}$ and $\rho_i(t) = 1/2N$ for any $i = 1, \cdots, 2N$, yielding min.$\{P(t)\} = 1/(2N)$, as shown explicitly in Fig. 2(bottom) of the main manuscript.

[1] A. Dutta, G. Aeppli, B. K. Chakrabarti, U. Divakaran, T. Rosenbaum, and D. Sen, *Quantum Phase Transitions in Transverse Field Spin Models: From Statistical Physics to Quantum Information* (Cambridge University Press, Cambridge, UK, 2015).
[2] T. Nag, V. Juričić, and B. Roy, Phys. Rev. Research **1**, 032045(R) (2019).
